# Supplementary material for: Thermal-fluctuator-driven decoherence of an oscillator near-resonantly coupled to a two-level system
Source: arXiv:2604.19322 source file (2026-11-28)
Supplement: Supplementary file 1 [file supp.tex]

\documentclass[12pt]{iopart}

\usepackage[utf8]{inputenc}
\usepackage[english]{babel}
\usepackage[LGR, T1]{fontenc}
\usepackage{amsmath}
\usepackage{float}
\usepackage{graphicx}
\usepackage{amsfonts}
\usepackage{amsthm}
\usepackage{amssymb}
\usepackage{etoolbox}
\usepackage[dvipsnames]{xcolor}
\usepackage{hyperref}
\usepackage{soul}
\usepackage{bbm}
\usepackage{commath}
\usepackage{enumerate}
\usepackage{mathtools} 
\usepackage{calrsfs}
\DeclareMathAlphabet{\pazocal}{OMS}{zplm}{m}{n}
\usepackage{upgreek}
\usepackage{calc}
\usepackage{accents}
\usepackage{siunitx}
\usepackage{color}
\usepackage{textcomp}
\usepackage{bm}
\usepackage{dsfont}
\usepackage{relsize}
\usepackage{braket}
\usepackage{enumitem}   
\usepackage{mathrsfs}
\usepackage[symbol]{footmisc}

\begin{document}

CONTAINS SUPPLEMENTARY INFORMATION

\section{Single two-level fluctuator}

Using the generic initial state expressed in terms of JC eigenstates, Eq.~\ref{eq: initial state}, and our knowledge of the JC eigenbasis, we can easily find the coherence measure at time $t$
\begin{equation}
\begin{aligned}
    C(t) = \frac{\mathrm{e}^{-i\omega_0t}}{\braket{\hat{a}(0)}}\sum_{\mu=\pm}p_\mu\Bigg\{c^*_0c_1\mathrm{e}^{-i(\delta + \mu\lambda)t}\,f_1(t) &+ \sum_{n=2}^\infty\sqrt{n}\,c_{n-1}^*c_n\,f_{n-1}(t)f_n(t) \\ & + \sum_{n=2}^\infty\sqrt{n-1}\,c_{n-1}^*c_n\,g_{n-1}(t)g_n(t)\Bigg\},
\end{aligned}
\end{equation}
where $f_n(t) = \cos\Omega^\mu_nt + i(\cos^2\vartheta_n^\mu - \sin^2\vartheta_n^\mu)\sin\Omega_n^\mu t$ and $g_n(t) = 2\left(\cos\vartheta_n^\mu\sin\vartheta_n^\mu\right)\sin\Omega^\mu_nt$ have been defined for compactness. This measure, in general, is quite complicated. However, for the simple superposition initial state, $\ket{\varphi_0} = (1/\sqrt{2})\{\ket{0} + \ket{1}\}$, we see that we have a considerable simplification and
\begin{equation}
    C(t) = \mathrm{e}^{-i\delta_+t/2}\sum_{\mu=\pm}p_\mu\mathrm{e}^{-i\mu\lambda t}\left\{\cos\Omega^\mu t + \frac{i\delta^\mu}{2\Omega^\mu}\sin\Omega^\mu t\right\},
\end{equation}
where we have defined $\Omega^\mu = \Omega^\mu_1$

\end{document}
